# Supplementary material for: Pinning induced motion and internal flow in neighbouring evaporating multi-component drops
Source: arXiv:2412.08495 source file (2025-06-20)

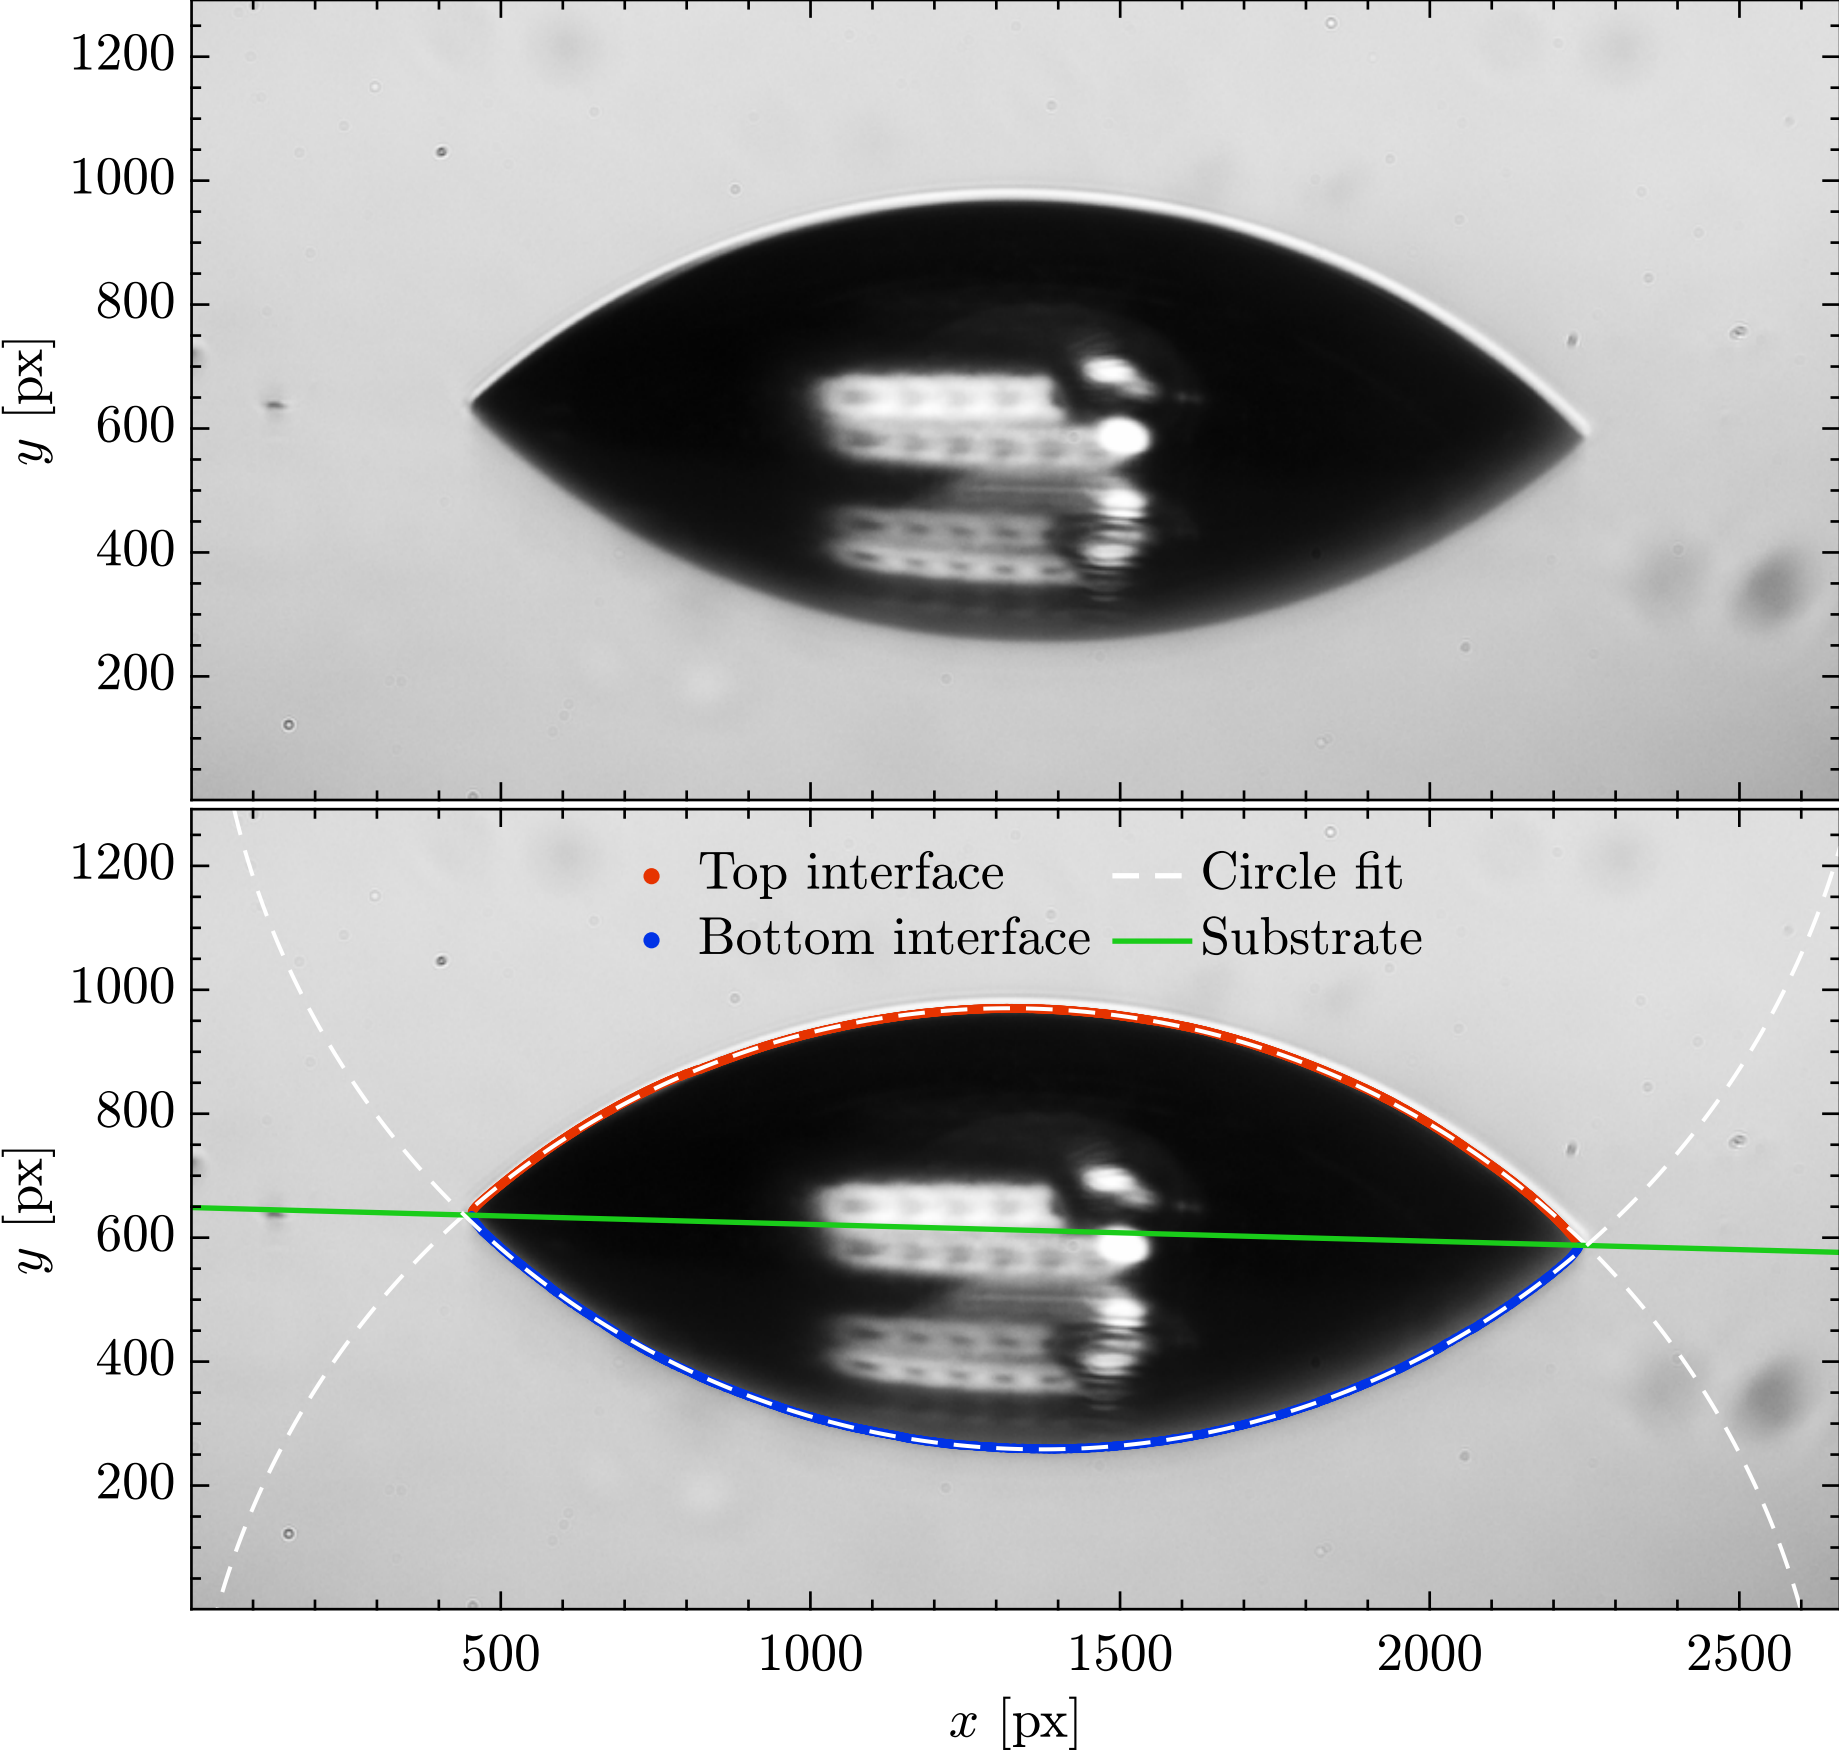

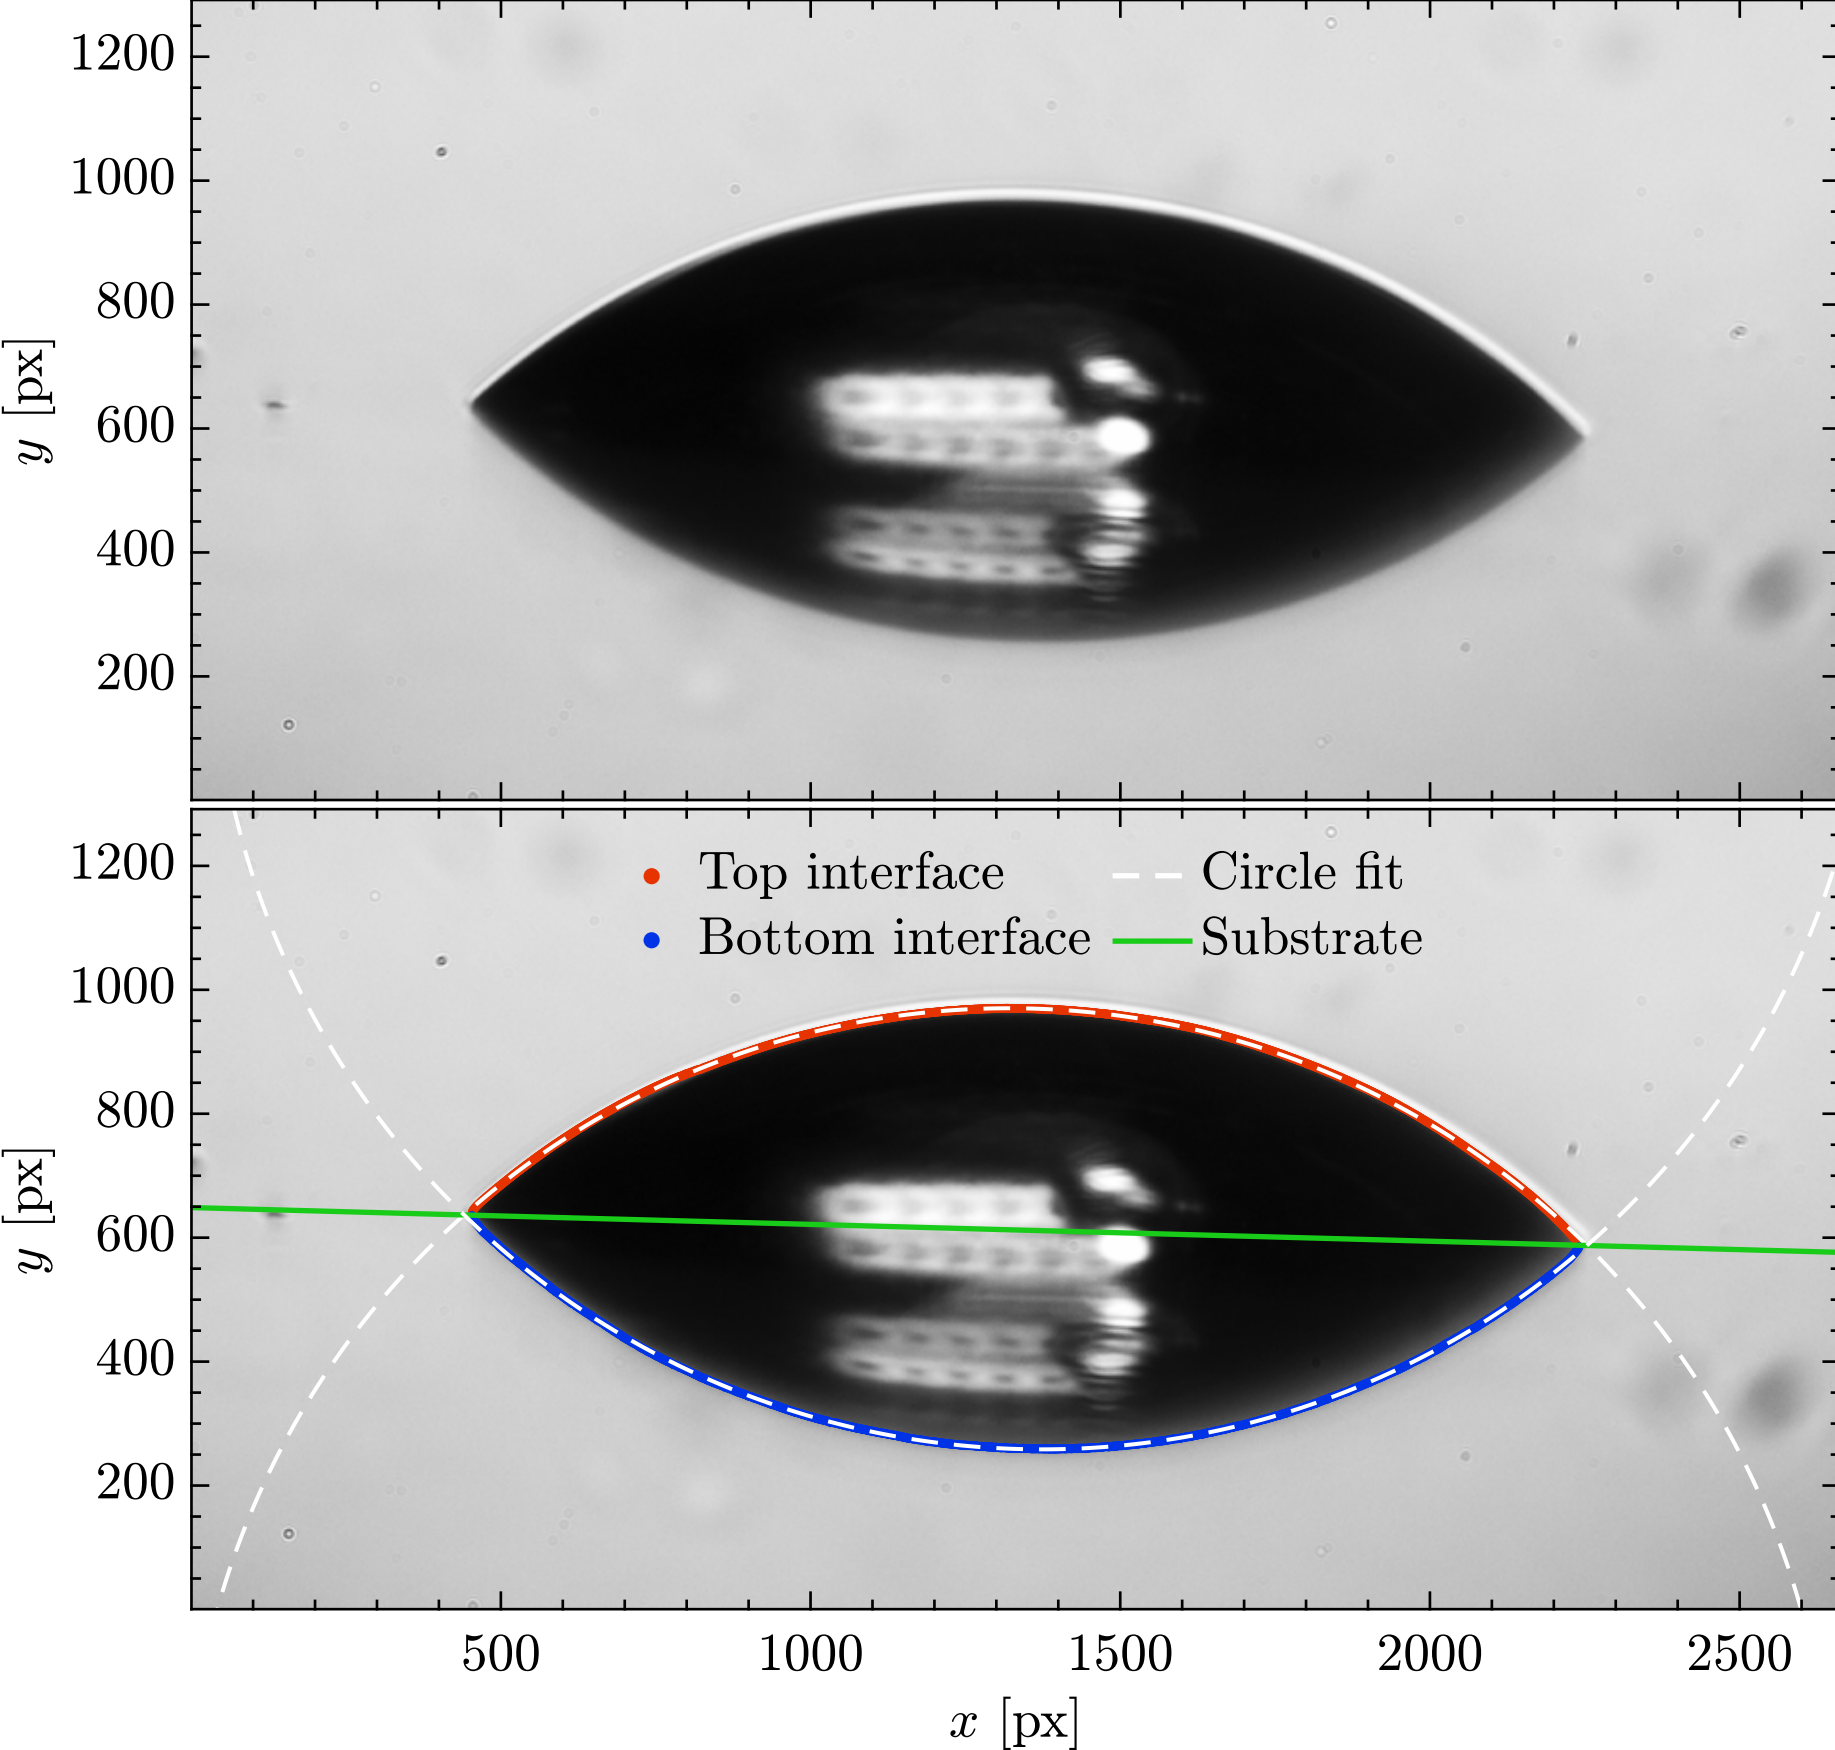

Supplement: Supplementary file 1 [file drop_circ_fit_k92_n15.pdf]
